# Supplementary material for: Spotting Suspicious Link Behavior with fBox: An Adversarial Perspective
Source: arXiv:1410.3915 source file (2014-10-15)
Supplement: Supplementary file 1 [file 090appendix.tex]

\section{Stealth appendix}
\reminder{here we put self notes etc}
